# Supplementary material for: 1-Lipschitz Layers Compared: Memory, Speed, and Certifiable Robustness
Source: arXiv:2311.16833 source file (2023-11-28)
Supplement: Supplementary file 1 [file appendix.tex]

\section{Gradient Analysis of Convex-Residual Layers}
\subsection{Basic Algebra Lemmas}
\begin{lem}
\label{lem:multi_distr}
Let $(G, \cdot, +)$ a ring with $1$ as identity for the product. For each $a_1,\ldots,a_n$, and for each $b$ the following holds
\begin{equation}
    \label{eq:multi_distr}
    (1+a_1)(1+a_2)\cdots(1+a_n)b=:\left(\prod_{i=1}^n(1+a_i) \right) b = b + \sum_{\substack{ 1\le k \le n \\
    1\le i_1<\cdots<i_k\le n}} a_{i_1}\cdots a_{i_k} b
\end{equation}
\begin{proof}
By induction over the number of factor $n$.\\
\textbf{P(n=1).} Equation~\ref{eq:multi_distr} coincides with the distributive property of the ring, formally
\begin{equation}
    (1+a_1)b= b + \sum_{\substack{ 1\le k \le 1 \\
    1\le i_1<\cdots<i_k\le 1}} a_{i_1}\cdots a_{i_k} b = b + a_1b
\end{equation}
\textbf{P(n-1)$\Rightarrow$ P(n)}. By applying the distributive property on the last factor, Equation~\ref{eq:multi_distr} split into the following
\begin{equation}
    \left(\prod_{i=1}^{n-1}(1+a_i) \right) (b + a_n b) =
    \left(\prod_{i=1}^{n-1}(1+a_i) \right)b + 
    \left(\prod_{i=1}^{n-1}(1+a_i) \right)a_n b 
\end{equation}
and, by assuming $\mathbf{P(n-1)}$, the right side of the previous formula can be written as follows
\begin{equation}
    \left[b + \sum_{\substack{ 1\le k \le n-1 \\
    1\le i_1<\cdots<i_k\le n-1}} a_{i_1}\cdots a_{i_k} b \right]+\left[ a_nb + \sum_{\substack{ 1\le k \le n-1 \\
    1\le i_1<\cdots<i_k\le n-1}} a_{i_1}\cdots a_{i_k} a_nb\right].
\end{equation}
Observe that the two summations can be joined into a single summation since the set of indexes have no intersection. This concludes the proof.
\end{proof}
\end{lem}

Lemma~\ref{lem:multi_distr} can be directly apply to explicit deduce the derivative of a residual neural network with respect to the inner weight, see later.

The growing popularity of $1-$Lipschitz neural networks push to consider a convex-relaxation of the residual term. For that specific case the following lemma will be useful.
\begin{lem}
\label{lem:multi_distr_scaled}
Let $(G,\cdot, +, \R)$ an algebra on the field of the real numbers with $e$ identity element of the $\cdot$ operation. Let $a_1,...,a_n$ and $b$ elements of $G$ and let $\alpha,\beta\in\R$. Then, the following identity holds
\begin{equation}
\left(\prod_{i=1}^n (\alpha e + \beta a_i)\right)b = \alpha^n b + \sum_{\substack{ 1\le k \le n \\
    1\le i_1<\cdots<i_k\le n}} \alpha^{n-k} \beta^k a_{i_1}\cdots a_{i_k} b 
\end{equation}
\begin{proof}
    TODO :)
\end{proof}
\end{lem}

\subsection{Derivatives of Residual Networks}
In this section we consider a real-case scenario of a residual network $f$ defined as a composition of $L$ residual layers $r^{(1)}, \ldots, r^{(L)}$ and a last layer $h^{(L+1)}$ 
\begin{equation}
    f(x) = h^{(L+1)} \circ r^{(L)} \circ \cdots \circ r^{(1)},
\end{equation}
where $y^{(i)} = r^{(i)}(y^{(i-1)}) = y^{(i-1)} + h^{(i)}(y^{(i-1)})$ and $h^{(i)}$ depends on and only the weight $\theta^{(i)}$.
Let assume $Loss:\R^n\times\R^c\to\R$ is the loss-function depending on the output of the network $y^{(L)} = f(x)$ and the ground truth vector $y$. The aim is to find the derivatives of the empirical risk over some distribution $(x,y)\sim\mu$ of an inner weight $\theta^{(l)}$ defined as 
\begin{equation}
    \LL(\theta) = \LL(\theta^{(L+1)},\theta^{(L)},\ldots,\theta^{(1)}) = \E_{(x,y)\sim \mu}\left[
        Loss(y^{(L+1)},y)
    \right].
\end{equation}

Let us write, for each $i=1,...,L$ the derivatives of $\LL$ with respect to the weight $\theta^{(i)}$,
\begin{equation}
    \begin{aligned}
    \frac{\partial \LL}{\partial \theta^{(l)}} &= \E\left[\frac{\partial Loss}{\partial y^{(L+1)}}\frac{\partial h^{(L+1)}}{\partial y^{(L)}}\frac{\partial r^{(L)}}{\partial y^{(L-1)}} \cdots \frac{\partial r^{(l+1)}}{\partial y^{(l)}}\frac{\partial r^{(l)}}{\partial \theta^{(l)}}\right] \\
    &= \E\left[\frac{\partial Loss}{\partial y^{(L+1)}}\frac{\partial h^{(L+1)}}{\partial y^{(L)}}
    \left(\prod_{l=1}^{L-l} \frac{\partial r^{(L-i+1)}}{\partial y^{(L-i)}}\right)\frac{\partial r^{(l)}}{\partial \theta^{(l)}}
    \right] \\
    &= \E\left[
    \frac{\partial Loss}{\partial y^{(L+1)}}
    \frac{\partial h^{(L+1)}}{\partial y^{(L)}}
    \left(
        \prod_{i=1}^{L-l} 
        I + 
        \frac{\partial h^{(L-i+1)}}{\partial y^{(L-i)}}
    \right)
    \frac{\partial h^{(l)}}{\partial \theta^{(l)}}
    \right].
    \end{aligned}
\end{equation}
By directly applying Lemma~\ref{lem:multi_distr} to the derivatives $a_i=\frac{\partial h^{(L-i+1)}}{\partial y^{(L-i)}}$ and $b=\frac{\partial h^{(l)}}{\partial \theta^{(l)}}$, previous formula can be reduced to the follows
\begin{equation}
\begin{aligned}
    \frac{\partial \LL}{\partial \theta^{(l)}}
    &= \E\left[
    \frac{\partial Loss}{\partial y^{(L+1)}}
    \frac{\partial h^{(L+1)}}{\partial y^{(L)}}
    \left(\frac{\partial h^{(l)}}{\partial \theta^{(l)}} +
        \sum_{\substack{1\le k \le L-l \\ 1\le i_1 < \ldots < i_k \le L-l}} \left( \prod_{j}^k\frac{\partial h^{(L-i_j+1)}}{\partial y^{(L-i_j)}}\right)\frac{\partial h^{(l)}}{\partial \theta^{(l)}}\right)
    \right] \\
    &= \E\left[
    \frac{\partial Loss}{\partial y^{(L+1)}}
    \frac{\partial h^{(L+1)}}{\partial y^{(L)}}
    \left(\frac{\partial h^{(l)}}{\partial \theta^{(l)}} +
        \sum_{\substack{1\le k \le L-l \\ 1\le i_1 < \ldots i_k \le L-l}} \left( \prod_{j}^k\frac{\partial h^{(L-i_j+1)}}{\partial y^{(L-i_j)}}\right)\frac{\partial h^{(l)}}{\partial \theta^{(l)}}\right)
    \right] \\
\end{aligned}
\end{equation}
\paragraph{Residual Networks with Convex Relaxation}
Neural networks with bounded Lipschitz constant are growing in popularity in the last few years from [Parseval] to [Anil] the constraint on the lipschitz constant can be obtaied in different ways. Recents works leverages Norm-Preserving layers deduced by orthgonal matrix and orthogonal convolutions. However, the performance of such a networks is far to be comparable to the state of the art neural networks for image classification. One of the theoretical motivations is given by [Bubeck], that roughly provide a lower bound on the number of parameters required in order to achive a good accuracy with 1-Lipschitz neural network. 

On the other side, training a large feed-forward neural is a tough task. As shown in previous section, residual networks instead can be trained without the effects of the vanishing gradient. Unfortunately, residual layers are not $1$ lispchitz, hence they can not be involved in a Lipscthiz bounded neural network. However, the following relaxation (namely \textit{convex relaxation}) can be applied to each residual layer in order to keep it 1-Lipschitz. From now on let assume that each residual $r^{(i)}$ depends on parameters $\theta^{(i)}$ and a scalar coefficient $\alpha_i\in[0,1]$ such that
\begin{equation}
    r^{(i)}(z) = \alpha_i z + (1 - \alpha_i)h^{(i)}(z)
\end{equation}

In the following analysis we aim at proving, in the milder assumption that $\alpha_1 = \cdots = \alpha_L = \alpha$,  that the derivatives of the convex relaxed-networks decays rapidly to $0$. Similarly to the previous analysis let
\begin{equation}
    f(x) = h^{(L+1)} \circ r^{(L)} \circ \cdots \circ r^{(1)},
\end{equation}
then the derivatives of the empirical risk $\LL(\theta)$ with respect to the weight $\theta^{(i)}$ can be written as follows
\begin{equation}
    \begin{aligned}
    \frac{\partial \LL}{\partial \theta^{(l)}} &= \E\left[\frac{\partial Loss}{\partial y^{(L+1)}}\frac{\partial h^{(L+1)}}{\partial y^{(L)}}\frac{\partial r^{(L)}}{\partial y^{(L-1)}} \cdots \frac{\partial r^{(l+1)}}{\partial y^{(l)}}\frac{\partial r^{(l)}}{\partial \theta^{(l)}}\right] \\
    &= \E\left[\frac{\partial Loss}{\partial y^{(L+1)}}\frac{\partial h^{(L+1)}}{\partial y^{(L)}}
    \left(\prod_{l=1}^{L-l} \frac{\partial r^{(L-i+1)}}{\partial y^{(L-i)}}\right)\frac{\partial r^{(l)}}{\partial \theta^{(l)}}
    \right] \\
    &= \E\left[
    \frac{\partial Loss}{\partial y^{(L+1)}}
    \frac{\partial h^{(L+1)}}{\partial y^{(L)}}
    \left(
        \prod_{i=1}^{L-l} 
        \alpha_i I + 
        (1-\alpha_i)\frac{\partial h^{(L-i+1)}}{\partial y^{(L-i)}}
    \right)
    \frac{\partial h^{(l)}}{\partial \theta^{(l)}}
    \right].
    \end{aligned}
\end{equation}

By directly applying Lemma~\ref{lem:multi_distr_scaled} to the derivatives $a_i=\frac{\partial h^{(L-i+1)}}{\partial y^{(L-i)}}$ and $b=\frac{\partial h^{(l)}}{\partial \theta^{(l)}}$ with $\alpha=\alpha_i$ and $\beta = (1-\alpha_i)$, previous formula can be reduced to the follows
\begin{equation}
\begin{aligned}
    \frac{\partial \LL}{\partial \theta^{(l)}}
    &= \E\left[
    \frac{\partial Loss}{\partial y^{(L+1)}}
    \frac{\partial h^{(L+1)}}{\partial y^{(L)}}
    \left(\alpha^{L-l}\frac{\partial h^{(l)}}{\partial \theta^{(l)}} +
        \sum_{\substack{1\le k \le L-l \\ 1\le i_1 < \ldots < i_k \le L-l}} \alpha^k\beta^{L-l-k}\left( \prod_{j}^k\frac{\partial h^{(L-i_j+1)}}{\partial y^{(L-i_j)}}\right)\frac{\partial h^{(l)}}{\partial \theta^{(l)}}\right)
    \right] \\
    &= \E\left[
    \frac{\partial Loss}{\partial y^{(L+1)}}
    \frac{\partial h^{(L+1)}}{\partial y^{(L)}}
    \left(\frac{\partial h^{(l)}}{\partial \theta^{(l)}} +
        \sum_{\substack{1\le k \le L-l \\ 1\le i_1 < \ldots i_k \le L-l}} \left( \prod_{j}^k\frac{\partial h^{(L-i_j+1)}}{\partial y^{(L-i_j)}}\right)\frac{\partial h^{(l)}}{\partial \theta^{(l)}}\right)
    \right] \\
\end{aligned}
\end{equation}
